# Supplementary material for: EASE: Entity-Aware Contrastive Learning of Sentence Embedding
Source: arXiv:2205.04260 source file (2022-05-09)
Supplement: Supplementary file 1 [file lareqa.tex]

\section{Cross-lingual QA Retrieval}
We evaluate multilingual sentence embeddings with a cross-lingual information retrieval task, LAReQA \citep{roy-etal-2020-lareqa}.
% Why this task?
This task is designed to measure strong alignment among languages: the model is asked to retrieve answer sentences from a multilingual candidate pool.
This means that the model needs to avoid ``language bias'', where a model prefers irrelevant answers in the question's language over correct results from another language.

% \paragraph{Model}
Following \citet{roy-etal-2020-lareqa}, all the models evaluated are the dual encoder model \citep{Gillick2018EndtoEndRI}.
The questions and answers are encoded as the pooled sentence embeddings from the pretrained model, and the candidate with the highest cosine similarity is retrieved as the answer.
The model is trained with the in-batch sampled softmax loss \citep{Henderson2017EfficientNL}.
We evaluate the models in the cross-lingual transfer setting, fine-tuning the models with the English SQuAD dataset \citep{rajpurkar-etal-2016-squad} and evaluate mean average precision (mAP) \citep{roy-etal-2020-lareqa} with $k=1000$.

% \paragraph{Results}
 Table \ref{table:lareqa} summarizes the results.
The EASE models consistently outperform the baselines, indicating that the multilingual sentence embeddings is also effective in the cross-lingual retrieval task with fine-tuning.

\begin{table}
\centering
\begin{tabular}{lc}\toprule
mBERT (avg.) & 27.4\\
mBERT (cls) & 29.2\\
SimCSE-mBERT\ba & 29.8\\
EASE-mBERT\ba & 29.8\\ \midrule
XLM-R (avg.) & 34.7\\
XLM-R (cls) & 34.6\\
SimCSE-XLM-R\ba & 35.1\\
EASE-XLM-R\ba & 35.4\\
\bottomrule
\end{tabular}
\caption{The mAP scores on the LAReQA dataset.}
\label{table:lareqa}
\end{table}
