# Supplementary material for: EASE: Entity-Aware Contrastive Learning of Sentence Embedding
Source: arXiv:2205.04260 source file (2022-05-09)
Supplement: Supplementary file 2 [file modularity.tex]

\section{Modularity}
\label{appendix:modularity}
In \cref{subsec:modularity}, we presented the modularity scores of Japanese-English parallel sentences from the Tatoeba dataset.
Here we present the results of the all 112 languages in the dataset in \Figure{fig:modularity-all}, plotting the modularity score for each language as well as the accuracy of parallel sentence matching.

Here, we can confirm the trends discussed in \cref{subsec:modularity}: SimCSE and EASE exhibit lower modularity scores than mBERT; LaBSE shows lowest modularity scores overall; and EASE shows higher modularity scores than SimCSE but performs better on parallel sentence matching.

Within a single model, we can see a clear pattern indicating that the lower the modularity score, the higher the accuracy of parallel sentence matching with different languages.
However, the comparison between SimCSE and EASE suggests that this does not necessarily hold when comparing different models.

\begin{figure}[h]

\begin{minipage}{.25\linewidth}
\centering
\subfloat[mBERT: 0.22 / 0.64.]{\label{fig:modularity-mBERT-all}\includegraphics[height=3.5cm]{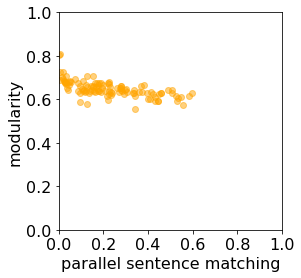}}
\end{minipage}\hfill
\begin{minipage}{.25\linewidth}
\centering
\subfloat[SimCSE: 0.23 / 0.49.]{\label{fig:modularity-SimCSE-all}\includegraphics[height=3.5cm]{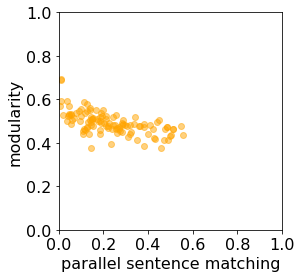}}
\end{minipage}\hfill
\begin{minipage}{.25\linewidth}
\centering
\subfloat[EASE: 0.33 / 0.53.]{\label{fig:modularity-EASE-all}\includegraphics[height=3.5cm]{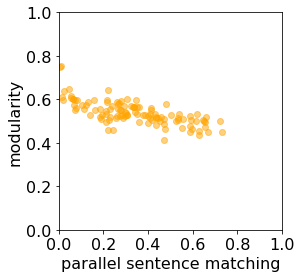}}
\end{minipage}\hfill
% \vspace{-1pt}
\begin{minipage}{.25\linewidth}
\centering
\subfloat[LaBSE: 0.83 / 0.17.]{\label{fig:modularity-LaBSE-all}\includegraphics[height=3.5cm]{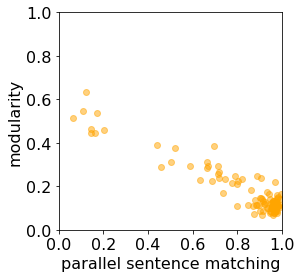}}
\end{minipage}
\caption{The accuracy scores of parallel sentence matching (x-axis) and modularity scores (y-axis) for all language pairs in the Tatoeba dataset. The values in the caption denotes (the average accuracy / the average modularity).}
\label{fig:modularity-all}
\end{figure}
