# Supplementary material for: EASE: Entity-Aware Contrastive Learning of Sentence Embedding
Source: arXiv:2205.04260 source file (2022-05-09)
Supplement: Supplementary file 3 [file monolingual_batch.tex]

\begin{table}
\centering
\begin{tabular}{lccc}
Model & mBERT & XLM-R \\ \hline
SimCSE (random) & 50.9 & 54.1 \\
SimCSE (mono) & 54.2 & 52.7 \\ \hline
EASE (random) & 57.2 & 57.1 \\
EASE (mono) & 53.7 & 54.2\\ \hline
\end{tabular}
\caption{mSTS}
\label{table: mono_batch}
\end{table}
